# Supplementary material for: Deep cross-domain building extraction for selective depth estimation from oblique aerial imagery
Source: arXiv:1804.08302 source file (2019-09-21)
Supplement: Supplementary file 1 [file 08_appendix.tex]

\section*{APPENDIX (Optional)}\label{Asec:appendix}

Any additional supporting data may be appended, provided the paper does not exceed the limits given above.
